# Supplementary material for: Deep Geometric Texture Synthesis
Source: arXiv:2007.00074 source file (2020-06-30)
Supplement: Supplementary file 1 [file appendix.tex]

\appendix
\appendix

\section{Line of Sight Projection}

Lets first consider the problem where we have a surface represented by Mesh $\hat{M1}$ and a set of viewers $ \{(\vec{p_i}, \vec{z_i})\}$ $p_i$ being the position of the viewer in space and $z_i$ the direction of sight from that point. We wish to draw all the lines of sights from all the points and decide whether they fall on the surface and all and if so where their intersection point is. For each face in $\hat{M1}$ corresponds a surface that can represented by an implicit function, where a point $\vec{r} \in \mathbb{R}^3$ is said to be on the plane if it satisfies the equation $\vec{n}\cdot\vec{r} + d = 0 $. where $\vec{n}$ is the surface normal and $d$ is a scalar. A point $\vec{r}$ is also said to be on the line of sight of viewer $i$ if exists a scalar $\alpha_i$ such that $\vec{r}=\alpha_i \vec{z_i} + \vec{p_i}$. It is relatively easy to see that plugging in the second equation into the first equation yields $\alpha_i=-1* \dfrac{d+\vec{n}\cdot\vec{p_i}}{\vec{n}\cdot\vec{z_i}}$. Now its only left to check whether the point $\hat{\vec{r_i}}=\alpha_i*\vec{z_i}+\vec{p_i}$ has fallen inside the triangular face, and this can be done in various ways. Calculation the sight intersections in this particular way can lead to one line of sight falling inside many triangular faces, it is only natural to take the face that is closest to $p_i$ to be a sight's projection.
This problem can also be relaxed to finding the point $\hat{\vec{r_i}}$ on each surface such that the product $l=  \dfrac{\hat{(\vec{r_i}} - \vec{p_i})\cdot\vec{z_i}}{\left\lVert (\vec{r_i} - \vec{p_i}) \right\rVert \left\lVert \vec{z_i} \right\rVert}$ is maximized.

Returning to the discrete problem, where we have points densely sampled from a surface, we can transfer the solution from continuous to discrete by taking the closest point $\vec{r_i}$ to $\vec{p_i}$ such that $l$ is larger than some threshold $cos(\epsilon)$ with epsilon being close to 0. Intuitively this takes to account all the points that could have been the sight intersection from $\vec{p_i}$ to the unknown surface, and picks the closest one to be the estimated point, very similarly to the continuous approach.
More analytically a bound in the probability sense for the number of input samples can be thought of in order to achieve a sight intersection.

Let $A$ be the entire surface area of the surface being reconstructed and lets assume the surface was uniformly sampled. If a point $p$ would have been with distance $L$ to the surface, the area of which a threshold $\epsilon$ would have been considered a valid projection points is $B = \pi L^2\cdot \tan{(\epsilon)}^2$. There for the probability $\delta$ for not finding any valid point is ought to be $\delta = {(1-\dfrac{A}{B})}^M$ where $M$ is the number of sample points from the surface. By applying the inequality $1 + t \leq e^t$ we get that $\delta \leq e^{-M\dfrac{A}{B}}$, with a little more manipulation we get 
\begin{gather*}
\dfrac{A \cdot \ln{(1/\delta)}}{B} \leq M \\
\dfrac{A \cdot\ln{(1/\delta)}}{=\pi \cdot min(L_i^2)\cdot \tan{(\epsilon)}^2} \leq M
\end{gather*}

It can be seen that if $min(L_i^2)$ goes to zero the whole expression goes to infinity regardless of $\delta$ or $\epsilon$. To combat this problem we try to eliminate projections from viewers who are really close to the surface, this is valid because if they are close enough to the surface the closest point to them is a fair approximation for their projection on the surface.
One method we found effective in our work to filter out such point is to calculate the knn between samples on the mesh, and viewers position, and the input point cloud, and filter out the points who are mutual knns to each other.

\section{Training Configurations}
